# Supplementary material for: hXDP: Efficient Software Packet Processing on FPGA NICs
Source: arXiv:2010.14145 source file (2020-10-27)
Supplement: Supplementary file 1 [file appendix-VLIW.tex]

\section{Superscalar vs VLIW architecture}

The entire design of \nxdp has the objective of maximizing performance while minimizing FPGA resources requirements. To achieve that, we do not include any runtime mechanism to optimize code execution, e.g., branch prediction, instruction re-ordering, etc. Instead, we rely on optimizations performed by the compiler, which statically performs any complex eBPF bytecode analysis and instruction-level optimization. This leads us towards designing a soft-CPU that implements a Very-Long-Instruction-Word (VLIW) architecture.

A VLIW processor can execute multiple instructions at the same time, like high-end superscalar server CPUs do, therefore it can take advantage of the instruction-level parallelism we discussed in Section~\ref{sec:instruction-analysis}. However, in the VLIW architecture the compiler is responsible to statically schedule instructions to the different VLIW processor's execution lanes. In a superscalar CPU, instead, the decision to run instructions in parallel is performed at runtime, with the processor dynamically checking the Bernstein's conditions continuously. 
Removing this capability from the processor greatly reduces the FPGA resources requirement. Intuitively, generalizing Bernstein's conditions for an arbitrary number of instructions, the number of comparisons required to check if the given instructions can run in parallel is given by:
\begin{equation}
    n_{checks} = 3 \times {{N}\choose{2}}
\end{equation}
Where $N$ is the number of instructions to parallelize. As $N \rightarrow \infty$, $n_{checks}$ grows as $O(N^2)$.
As we have seen in Section~\ref{sec:perf_eval}, despite performing only static checks, the \nxdp istruction-per-cycle rate is similar to that achieved by more complex sever-level CPUs while using very little hardware resources.
