# Supplementary material for: hXDP: Efficient Software Packet Processing on FPGA NICs
Source: arXiv:2010.14145 source file (2020-10-27)
Supplement: Supplementary file 2 [file appendix-apps.tex]

\subsection{Katran}
Katran~\cite{katran} is a high performance SW load balancer framework based on a C++ library and two eBPF kernel modules. The Katran eBPF module exposes a set of virtual IP addresses (\emph{VIP}) identified as an (IP address, port) pair and it associates a set of real servers IP addresses (\emph{REALs}) to each VIP. Upon receipt of the first packet of a flow directed to one of the registered VIPs (which are stored in a hash map), Katran picks one of the reals according to a simple weighted scheduling policy. The association between the flow 5-tuple and the corresponding REAL is stored in a per-CPU LRU hash map so that all the subsequent packets belonging to the same flow will be associated to the same REAL. As soon as the corresponding REAL is identified, Katran encapsulates the received packets in an IPinIP tunnel toward the REAL and it updates a set of metrics stored in a set of array maps. Katran works in direct response mode, meaning that the response packets from the REALs are sent directly to the corresponding clients without being intercepted and processed by Katran. Katran also includes an optional IPinIP health check module to monitor REALs' availability. For the evaluation of our work this module is turned off.
